# Supplementary material for: Multimodal Contextualized Plan Prediction for Embodied Task Completion
Source: arXiv:2305.06485 source file (2023-05-10)
Supplement: Supplementary file 1 [file exec_stats.tex]

Model = gt, Plan exec method = direct, Frac nav failures = 12 / 1460 = 0.82
Fraction of obj interaction failures = %s [('Place__Cabinet', 100.0), ('Pour__Pot', 100.0), ('Open__Cabinet', 90.48), ('Place__StoveBurner', 87.5), ('ToggleOff__Stove
Knob', 81.82), ('Place__Floor', 71.43), ('Slice__Lettuce', 58.82), ('Open__Drawer', 55.56), ('Pickup__Tomato', 53.85), ('Pickup__Pot', 50.0), ('Place__CoffeeTable', 5
0.0), ('Pickup__SoapBottle', 50.0), ('Pickup__Potato', 45.0), ('Place__Plate', 43.48), ('Pickup__LettuceSliced', 41.18), ('Place__Pot', 40.0), ('Pickup__Bread', 38.46
), ('Pickup__Lettuce', 37.5), ('ToggleOn__StoveKnob', 36.36), ('Slice__Bread', 35.71), ('Pickup__TomatoSliced', 35.71), ('Place__DiningTable', 34.09), ('Pickup__DishS
ponge', 33.33), ('Pickup__Apple', 33.33), ('Pickup__Spatula', 33.33), ('Place__SinkBasin', 30.56), ('Pickup__PepperShaker', 30.0), ('Slice__Tomato', 26.32), ('Pickup_
_ButterKnife', 25.0), ('Slice__Potato', 25.0), ('Place__Sink', 25.0), ('Pickup__SaltShaker', 25.0), ('Pickup__Spoon', 25.0), ('Pickup__Plate', 23.53), ('Place__Counte
rTop', 22.04), ('Place__Toaster', 21.05), ('Pickup__Mug', 20.51), ('Pour__Sink', 20.0), ('Pickup__Fork', 20.0), ('Pickup__Egg', 20.0), ('Place__Pan', 18.18), ('Pickup
__Knife', 17.02), ('Pickup__RemoteControl', 16.67), ('Pickup__Pan', 16.67), ('Pour__HousePlant', 16.67), ('Pour__SinkBasin', 16.0), ('Place__Microwave', 14.29), ('Pla
ce__Sofa', 14.29), ('Pickup__BreadSliced', 13.11), ('Place__CoffeeMachine', 12.5), ('Close__Fridge', 12.5), ('Pickup__Bowl', 11.11), ('Place__Bowl', 10.0), ('ToggleOf
f__Microwave', 9.09), ('Close__Cabinet', 9.09), ('ToggleOn__Faucet', 7.89), ('Open__Microwave', 7.14), ('Close__Microwave', 7.14), ('Pickup__PotatoSliced', 6.12), ('T
oggleOff__Faucet', 3.57), ('ToggleOn__Microwave', 0.0), ('ToggleOn__CoffeeMachine', 0.0), ('ToggleOff__CoffeeMachine', 0.0), ('ToggleOn__Toaster', 0.0), ('Open__Fridg
e', 0.0), ('ToggleOff__Toaster', 0.0), ('Place__Dresser', 0.0), ('Pickup__Cloth', 0.0), ('Place__BathtubBasin', 0.0), ('Pickup__WineBottle', 0.0), ('Place__Fridge', 0
.0), ('Place__ArmChair', 0.0), ('Close__Drawer', 0.0), ('Pickup__Pillow', 0.0), ('Pickup__Newspaper', 0.0), ('Pickup__Cup', 0.0), ('Pickup__Watch', 0.0), ('Place__Sid
eTable', 0.0), ('Pickup__Ladle', 0.0), ('Place__Desk', 0.0), ('Pickup__AlarmClock', 0.0), ('Pickup__SprayBottle', 0.0), ('Pickup__TissueBox', 0.0), ('Pickup__PaperTow
elRoll', 0.0), ('Pickup__Pencil', 0.0), ('Pickup__CreditCard', 0.0)]

Model = gt, Plan exec method = ea, Frac nav failures = 16 / 1542 = 1.04
Fraction of obj interaction failures = %s [('Place__StoveBurner', 75.0), ('Open__Drawer', 66.67), ('Open__Cabinet', 52.43), ('Place__CoffeeTable', 50.0), ('Pickup__So
apBottle', 50.0), ('Slice__Lettuce', 42.86), ('Open__Microwave', 38.71), ('Place__Plate', 37.29), ('Pickup__Bread', 33.33), ('Place__Dresser', 33.33), ('Pickup__Pot',
 29.41), ('Pickup__LettuceSliced', 28.21), ('Pickup__Lettuce', 27.27), ('Pickup__Potato', 25.58), ('Place__ArmChair', 25.0), ('Place__Pot', 25.0), ('Pickup__TomatoSli
ced', 24.14), ('Pickup__Knife', 24.07), ('Place__SinkBasin', 22.22), ('Close__Cabinet', 21.43), ('ToggleOff__Microwave', 20.0), ('Pour__Sink', 20.0), ('Pickup__Tomato
', 20.0), ('Place__Floor', 20.0), ('Pickup__Mug', 18.6), ('Close__Fridge', 18.18), ('Slice__Bread', 18.18), ('Slice__Tomato', 17.65), ('Pickup__PepperShaker', 16.67),
 ('Pickup__RemoteControl', 16.67), ('Pickup__Cloth', 16.67), ('Pour__HousePlant', 16.67), ('Pickup__Apple', 16.67), ('Pour__SinkBasin', 16.0), ('Place__CounterTop', 1
5.3), ('Pickup__ButterKnife', 14.29), ('Place__DiningTable', 11.43), ('Place__Toaster', 11.11), ('Place__Bowl', 10.53), ('Pickup__BreadSliced', 10.45), ('ToggleOn__St
oveKnob', 10.0), ('Pickup__Plate', 8.62), ('Slice__Potato', 8.33), ('Pickup__PotatoSliced', 6.9), ('Place__CoffeeMachine', 6.67), ('Pickup__Bowl', 6.06), ('ToggleOn__
Faucet', 5.26), ('Place__Microwave', 0.0), ('Close__Microwave', 0.0), ('ToggleOn__Microwave', 0.0), ('ToggleOn__CoffeeMachine', 0.0), ('Place__Sink', 0.0), ('ToggleOf
f__Faucet', 0.0), ('ToggleOff__CoffeeMachine', 0.0), ('Pickup__SaltShaker', 0.0), ('ToggleOn__Toaster', 0.0), ('Open__Fridge', 0.0), ('ToggleOff__Toaster', 0.0), ('Op
en__Toilet', 0.0), ('Place__BathtubBasin', 0.0), ('Pickup__Fork', 0.0), ('Pickup__Spoon', 0.0), ('Pickup__WineBottle', 0.0), ('Place__Fridge', 0.0), ('Pickup__Pan', 0
.0), ('ToggleOff__StoveKnob', 0.0), ('Close__Drawer', 0.0), ('Pickup__DishSponge', 0.0), ('Pickup__Pillow', 0.0), ('Place__Sofa', 0.0), ('Pickup__Newspaper', 0.0), ('Place__Cabinet', 0.0), ('Pickup__Egg', 0.0), ('Pickup__Cup', 0.0), ('Pickup__Watch', 0.0), ('Place__SideTable', 0.0), ('Pickup__Ladle', 0.0), ('Place__Pan', 0.0), ('$lace__Desk', 0.0), ('Pickup__AlarmClock', 0.0), ('Pickup__SprayBottle', 0.0), ('Pickup__Spatula', 0.0), ('Pickup__TissueBox', 0.0), ('Pickup__PaperTowelRoll', 0.0), $'Pickup__Pencil', 0.0), ('Pickup__CreditCard', 0.0)]

Model = gt_coref, Plan exec method = direct, Frac nav failures = 9 / 1456 = 0.62
Fraction of obj interaction failures = %s [('Open__Drawer', 100.0), ('Pour__Pot', 100.0), ('Place__StoveBurner', 75.0), ('Place__Cabinet', 66.67), ('Place__Floor', 57.14), ('Pickup__Cup', 50.0), ('Place__CoffeeTable', 50.0), ('Pickup__SoapBottle', 50.0), ('Pour__Sink', 40.0), ('Open__Cabinet', 38.1), ('Place__DiningTable', 37.21), ('Place__SinkBasin', 33.33), ('Pickup__Newspaper', 33.33), ('Pickup__TomatoSliced', 32.14), ('Place__Plate', 27.54), ('Place__ArmChair', 25.0), ('Pickup__Pot', 25.0), ('Slice__Lettuce', 23.53), ('Pickup__Tomato', 23.08), ('Slice__Bread', 21.43), ('Pickup__LettuceSliced', 21.21), ('Pickup__Potato', 20.51), ('Pickup__PepperShaker', 20.0), ('Pickup__Fork', 20.0), ('Place__Pot', 20.0), ('Pickup__Bread', 18.18), ('Place__Pan', 18.18), ('Pickup__RemoteControl', 16.67), ('Pickup__Pan', 16.67), ('Pickup__Apple', 16.67), ('Pour__SinkBasin', 16.0), ('Place__Bowl', 15.0), ('Place__Microwave', 14.29), ('Place__Sofa', 14.29), ('Pickup__Mug', 12.82), ('Pickup__SaltShaker', 12.5), ('Close__Fridge', 12.5), ('Pickup__Lettuce', 12.5), ('Pickup__PotatoSliced', 12.0), ('Pickup__Plate', 11.76), ('Pickup__BreadSliced', 11.48), ('Place__CounterTop', 11.02), ('Slice__Tomato', 10.53), ('Pickup__ButterKnife', 10.0), ('Pickup__Egg', 10.0), ('ToggleOff__Microwave', 9.09), ('ToggleOn__StoveKnob', 9.09), ('Pickup__Knife', 8.51), ('ToggleOn__Faucet', 7.89), ('Open__Microwave', 7.14), ('Close__Microwave', 7.14), ('Place__Toaster', 5.26), ('Pickup__Bowl', 3.7), ('ToggleOff__Faucet', 3.57), ('Slice__Potato', 0.0), ('ToggleOn__Microwave', 0.0), ('Place__CoffeeMachine', 0.0), ('ToggleOn__CoffeeMachine', 0.0), ('Place__Sink', 0.0), ('ToggleOff__CoffeeMachine', 0.0), ('ToggleOn__Toaster', 0.0), ('Open__Fridge', 0.0), ('ToggleOff__Toaster', 0.0), ('Place__Dresser', 0.0), ('Close__Cabinet', 0.0), ('Pickup__Cloth', 0.0), ('Place__BathtubBasin', 0.0), ('Pickup__Spoon', 0.0), ('Pickup__WineBottle', 0.0), ('Place__Fridge', 0.0), ('ToggleOff__StoveKnob', 0.0), ('Close__Drawer', 0.0), ('Pour__HousePlant', 0.0), ('Pickup__DishSponge', 0.0), ('Pickup__Pillow', 0.0), ('Pickup__Watch', 0.0), ('Place__SideTable', 0.0), ('Pickup__Ladle', 0.0), ('Place__Desk', 0.0), ('Pickup__AlarmClock', 0.0), ('Pickup__SprayBottle', 0.0), ('Pickup__Spatula', 0.0), ('Pickup__TissueBox', 0.0), ('Pickup__PaperTowelRoll', 0.0), ('Pickup__Pencil', 0.0), ('Pickup__CreditCard', 0.0)]

Model = gt_coref, Plan exec method = ea, Frac nav failures = 11 / 1491 = 0.74
Fraction of obj interaction failures = %s [('Place__StoveBurner', 100.0), ('Pour__Pot', 100.0), ('Open__Cabinet', 53.45), ('Place__Dresser', 50.0), ('Place__CoffeeTable', 50.0), ('Pickup__SoapBottle', 50.0), ('Open__Microwave', 42.86), ('Pickup__Cup', 42.86), ('Pour__Sink', 40.0), ('Open__Drawer', 40.0), ('ToggleOn__StoveKnob', 36.36), ('Close__Cabinet', 35.29), ('Place__ArmChair', 33.33), ('Place__Pot', 33.33), ('Pickup__Newspaper', 33.33), ('Pickup__Potato', 24.39), ('Pickup__TomatoSliced', 24.14), ('ToggleOff__Microwave', 23.08), ('Pickup__Lettuce', 22.22), ('Pickup__RemoteControl', 20.0), ('Place__Floor', 20.0), ('Pickup__Plate', 19.3), ('Place__Plate', 18.64), ('Close__Fridge', 17.65), ('Pickup__Cloth', 16.67), ('Pickup__Apple', 16.67), ('Place__SinkBasin', 15.62), ('Pickup__Tomato', 15.38), ('Pickup__LettuceSliced', 14.71), ('Pickup__Pot', 14.29), ('Place__DiningTable', 13.89), ('Pickup__Mug', 12.2), ('Pickup__Knife', 12.0), ('Place__Bowl', 10.53), ('Pickup__ButterKnife', 10.0), ('Pickup__PepperShaker', 10.0), ('Pickup__BreadSliced', 9.38), ('Pickup__Bread', 9.09), ('Place__Pan', 9.09), ('Place__CounterTop', 8.53), ('Pour__SinkBasin', 8.0), ('Pickup__PotatoSliced', 7.55), ('Slice__Lettuce', 7.14), ('Slice__Tomato', 5.56), ('Pickup__Bowl', 3.23), ('ToggleOn__Faucet', 2.63), ('ToggleOff__Faucet', 1.72), ('Place__Toaster', 0.0), ('Slice__Potato', 0.0), ('Place__Microwave', 0.0), ('Close__Microwave', 0.0), ('ToggleOn__Microwave', 0.0), ('Place__CoffeeMachine', 0.0), ('ToggleOn__CoffeeMachine', 0.0), ('Place__Sink', 0.0), ('ToggleOff__CoffeeMachine', 0.0), ('Pickup__SaltShaker', 0.0), ('Slice__Bread', 0.0), ('ToggleOn__Toaster', 0.0), ('Open__Fridge', 0.0), ('ToggleOff__Toaster', 0.0), ('Open__Toilet', 0.0), ('Place__BathtubBasin', 0.0), ('Pickup__Fork', 0.0), ('Pickup__Spoon', 0.0), ('Pickup__WineBottle', 0.0), ('Place__Fridge', 0.0), ('ToggleOff__StoveKnob', 0.0), ('Pickup__Pan', 0.0), ('Close__Drawer', 0.0), ('Pour__HousePlant', 0.0), ('Pickup__DishSponge', 0.0), ('Pickup__Pillow', 0.0), ('Place__Sofa', 0.0), ('Place__Cabinet', 0.0), ('Pickup__Egg', 0.0), ('Pickup__Watch', 0.0), ('Place__SideTable', 0.0), ('Pickup__Ladle', 0.0), ('Place__Desk', 0.0), ('Pickup__AlarmClock', 0.0), ('Pickup__SprayBottle', 0.0), ('Pickup__Spatula', 0.0), ('Pickup__TissueBox', 0.0), ('Pickup__PaperTowelRoll', 0.0), ('Pickup__Pencil', 0.0), ('Pickup__CreditCard', 0.0)]
